# Supplementary material for: Decoding Shake-up Satellites in XPS through Large-Scale ab initio Simulations: Spectral Signatures of Ring Fusion in Porphyrins
Source: arXiv:2509.26057 ancillary file (2025-09-30)
Supplement: Supplementary file 1 [file supporting_information.pdf]

# Supporting Information: Decoding Shake-up Satellites in XPS through Large-Scale ab initio Simulations: Spectral Signatures of Ring Fusion in Porphyrins

Jannis Kockläuner,<sup>\*,†</sup> Majid Shaker,<sup>‡</sup> Maximilian Muth,<sup>‡</sup> Simon Steinbach,<sup>‡</sup>  
Christoph Oleszak,<sup>¶</sup> Ole Lytken,<sup>‡</sup> Hans-Peter Steinrück,<sup>‡</sup> and Dorothea  
Golze<sup>\*,†</sup>

<sup>†</sup>*Faculty of Chemistry and Food Chemistry, Technische Universität Dresden, 01062 Dresden,  
Germany*

<sup>‡</sup>*Chair of Physical Chemistry II, Friedrich-Alexander-Universität Erlangen-Nürnberg,  
Egerlandstr. 3, 91058 Erlangen, Germany*

<sup>¶</sup>*Chair of Organic Chemistry II, Friedrich-Alexander-Universität Erlangen-Nürnberg,  
Nikolaus-Fiebiger-Str. 10, 91058 Erlangen, Germany*

E-mail: jannis.kocklaeuner@tu-dresden.de; dorothea.golze@tu-dresden.de

## S1 Additional Computational Details

We performed all-electron  $G_{\Delta H}W_0$  and  $GW + C$  calculations for molecules **1-4** using the FHI-aims program package<sup>S1-S3</sup> following the workflow of Ref. S4.  $G_{\Delta H}W_0$  denotes the inclusion of the Hedin shift in the  $G_0W_0$  framework as explained in Ref. S5. The geometries of molecules **1-4** were optimized at the DFT level using numeric atom-centred orbitals of *tier 2* quality (FHI-aims-2020

default). We employed the PBE exchange-correlation functional<sup>S6</sup> including van-der-Waals interactions via the Tkatchenko-Scheffler dispersion correction<sup>S7</sup> and scalar-relativistic effects using the atomic zeroth order regular approximation.<sup>S1</sup> Structures **5** and **6** were derived from compounds **3** and **4**, respectively, by replacing *tert*-butyl groups with hydrogen atoms, without further geometry optimization.

We used the PBE functional as the starting point for  $G_{\Delta H}W_0$  calculations and applied the contour deformation technique with analytical continuation of  $W$  (CD-WAC) for frequency integration.<sup>S8,S9</sup> The integration along the imaginary axis was carried out using a 200-point modified Gauss-Legendre grid. In the CD-WAC approach,  $W_{mn}^c$  was evaluated at 300 reference frequencies: 200 imaginary points from the Gauss-Legendre grid and 100 additional real frequencies split between the core (80) and valence (20) regions (see Ref. S9). We employed the FHI-aims-2020 *tier 2* basis set (T2), augmented with two diffuse functions (+aug2) taken from the  $l = 0, 1$  augmentation functions of the aug-cc-pV5Z basis set.<sup>S10</sup> For nitrogen atoms, we added localized Slater-type orbitals (STO2) with maximum principal quantum number  $n = 2$ .<sup>S11</sup>

For compounds **1**, **5**, and **6**, the exact analytical transition moments  $\rho_{1s,1s}^\nu$  and satellite intensities  $\gamma^\nu$  were computed by solving the Casida equation Eq. 7. We used energy thresholds of  $\epsilon_i > -2 E_H$  and  $\epsilon_a < 3 E_H$  to truncate the states included in the construction of the matrix elements  $A_{ia,jb}$  and  $B_{ia,jb}$  to reduce the computational cost. The T2+aug2 basis set without additional STO functions was used, as it provides essentially the same satellite spectra.<sup>S4,S12-S14</sup> In addition, we computed the optical absorption spectrum of **1** by solving the full Bethe-Salpeter equation based on an eigenvalue-self-consistent GW starting point (BSE@evGW), as implemented in the Turbomole package.<sup>S15</sup> We used the recommended def2-TZVP basis set and the default settings in the evGW step. For the BSE calculation, we chose to freeze the 48 1s core-orbitals as well as the 1000 virtual orbitals with the highest energy. Transition densities  $n_\nu(\mathbf{r})$  were calculated in a post-processing step by summing contributions with RPA eigenvector coefficients  $|X_{ia}^\nu + Y_{ia}^\nu|^2 > 0.01$ . All transition densities are plotted using a isosurface value of  $\pm 0.003$ .

## S2 Tracing the origin of shake-up satellites: Mono-fused system **5**

Here, we provide a similar analysis as in section 4.2 of the main text for compound **5**. In Figure S1, we show the optical RPA spectrum (black) alongside the individual satellite spectra. For comparison, the broadened  $GW + C$  spectral functions of **3** are shown in gray.

For the optical spectrum, we observe that the spectrum is dominated by an intense transition at 2.9 eV ( $S_8$ , see Table S1). Although the peak resembles the Soret ( $B_{x/y}$ ) band in **1**, we note that the pattern of the interacting orbitals does not match the Gouterman model, instead it is mainly due to a transition from HOMO-4 $\rightarrow$ LUMO. At higher energies, we find several excitations with similar contributions between 3.2 and 4.0 eV.

For the satellite spectrum, we observe that we can group the spectra roughly into pairs of two, the N1/N2 levels with intensity maxima around 3.4 eV, and the N3/N4 levels with intensity maxima around 2.5 eV. The N1/N2 shake-up spectra show an intense peak due to the  $S_1$  transition, which is absent from the N3/N4 levels. The maximum intensity of the N1/N2 satellite spectrum is around 3.4 eV, with several transitions contributing significant spectral weight. The maximum of the N3 spectrum is around 2.4 eV and is dictated by the intense  $S_4$  transition, while the dominant contribution to the N4 spectrum comes from the  $S_7$  excitation.

Compared to the broadened spectrum of the parent compound **3** (gray shaded area), we observe that the maxima coincide reasonably well within ca. 0.3 eV with the satellite spectrum of **5** for all core levels. We note that the intense  $S_1$  transition is observed in the N1 spectrum of **3**, while it appears to be absent in the N2 spectrum, which will be discussed in more detail in section S3.

In Figure S2, we show the transition densities of the lowest 12 RPA excitations of **5**. The symmetry breaking induced by the ring fusion breaks the initial approximate  $D_{2h}$  symmetry of the macrocycle, and therefore we cannot exclude any shake-up states based on symmetry arguments. Therefore, the intensity is solely dictated by the local sign and magnitude of the transition density around the core level. As an example, the  $S_7$  transition is strongly localized with the same phase in the vicinity of the N3 and N4 core, while it has no density in the region of the N1 and N2

cores. Consequently, we observe intense  $S_7$  shake-up excitations for the N3 and N4 core, while it is absent in the spectra of the N1 and N2 core levels.

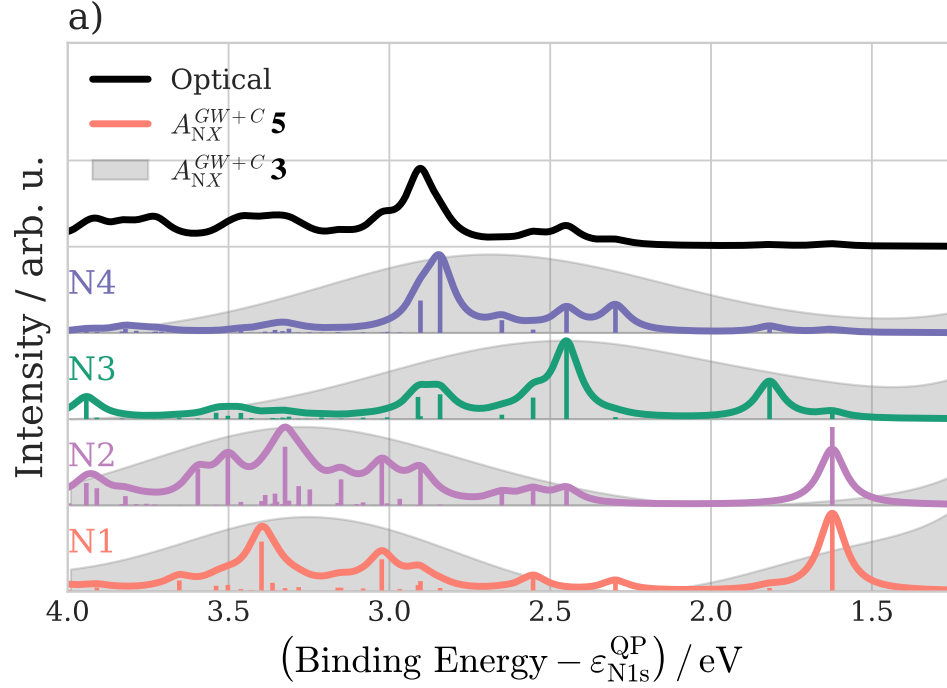

**Figure S1:** Direct comparison of the first-order N1s satellite spectra (colored lines) of all N1s states with the optical absorption spectra (black line). Individual satellite intensities  $\gamma_{N1s}^\nu$  are shown as stick spectrum. The maximum of each spectrum is set to the same value to enable comparison. The respective  $GW + C$  satellite spectra of **4** (from Figure 2 of the main text) are shown in gray as reference.

**Table S1:** RPA excitation energies  $\Omega^\nu$ , oscillator strengths  $f^\nu$  and  $GW + C$  satellite intensities  $\gamma_{N_X}^\nu$  of the 30 lowest energy singlet excitations in **5**.

| $\nu$ | $\Omega^\nu / \text{eV}$ | $f^\nu$ | $\gamma_{N1}^\nu$ | $\gamma_{N2}^\nu$ | $\gamma_{N3}^\nu$ | $\gamma_{N4}^\nu$ |
|-------|--------------------------|---------|-------------------|-------------------|-------------------|-------------------|
| 1     | 1.6231                   | 0.0256  | 0.0409            | 0.0258            | 0.0049            | 0.0038            |
| 2     | 1.8180                   | 0.0143  | 0.0019            | 0.0001            | 0.0312            | 0.0078            |
| 3     | 2.2971                   | 0.0470  | 0.0053            | 0.0000            | 0.0016            | 0.0319            |
| 4     | 2.4492                   | 0.1842  | 0.0000            | 0.0067            | 0.0616            | 0.0270            |
| 5     | 2.5532                   | 0.0958  | 0.0076            | 0.0054            | 0.0170            | 0.0035            |
| 6     | 2.6503                   | 0.0245  | 0.0005            | 0.0040            | 0.0035            | 0.0134            |
| 7     | 2.8423                   | 0.1670  | 0.0019            | 0.0002            | 0.0195            | 0.0823            |
| 8     | 2.9033                   | 0.5515  | 0.0055            | 0.0133            | 0.0023            | 0.0340            |
| 9     | 2.9110                   | 0.1658  | 0.0034            | 0.0001            | 0.0175            | 0.0000            |
| 10    | 2.9677                   | 0.0216  | 0.0013            | 0.0022            | 0.0000            | 0.0004            |
| 11    | 3.0066                   | 0.0066  | 0.0001            | 0.0007            | 0.0014            | 0.0011            |
| 12    | 3.0235                   | 0.1924  | 0.0169            | 0.0145            | 0.0002            | 0.0004            |
| 13    | 3.0445                   | 0.0125  | 0.0000            | 0.0001            | 0.0001            | 0.0001            |
| 14    | 3.0817                   | 0.0029  | 0.0016            | 0.0010            | 0.0012            | 0.0006            |
| 15    | 3.1019                   | 0.0049  | 0.0005            | 0.0004            | 0.0000            | 0.0000            |
| 16    | 3.1501                   | 0.0397  | 0.0020            | 0.0086            | 0.0004            | 0.0003            |
| 17    | 3.1603                   | 0.0301  | 0.0021            | 0.0008            | 0.0000            | 0.0009            |
| 18    | 3.2108                   | 0.0046  | 0.0005            | 0.0000            | 0.0013            | 0.0004            |
| 19    | 3.2229                   | 0.0007  | 0.0000            | 0.0000            | 0.0001            | 0.0001            |
| 20    | 3.2472                   | 0.0164  | 0.0001            | 0.0053            | 0.0001            | 0.0007            |
| 21    | 3.2499                   | 0.0009  | 0.0001            | 0.0003            | 0.0000            | 0.0002            |
| 22    | 3.2597                   | 0.0003  | 0.0000            | 0.0000            | 0.0002            | 0.0000            |
| 23    | 3.2819                   | 0.0642  | 0.0023            | 0.0063            | 0.0003            | 0.0002            |
| 24    | 3.2837                   | 0.0007  | 0.0000            | 0.0004            | 0.0000            | 0.0003            |
| 25    | 3.2953                   | 0.0177  | 0.0002            | 0.0000            | 0.0001            | 0.0003            |
| 26    | 3.3122                   | 0.0427  | 0.0003            | 0.0016            | 0.0020            | 0.0044            |
| 27    | 3.3243                   | 0.0503  | 0.0018            | 0.0193            | 0.0005            | 0.0005            |
| 28    | 3.3321                   | 0.0321  | 0.0000            | 0.0004            | 0.0012            | 0.0019            |
| 29    | 3.3496                   | 0.0106  | 0.0001            | 0.0012            | 0.0005            | 0.0005            |
| 30    | 3.3555                   | 0.0078  | 0.0008            | 0.0039            | 0.0001            | 0.0031            |

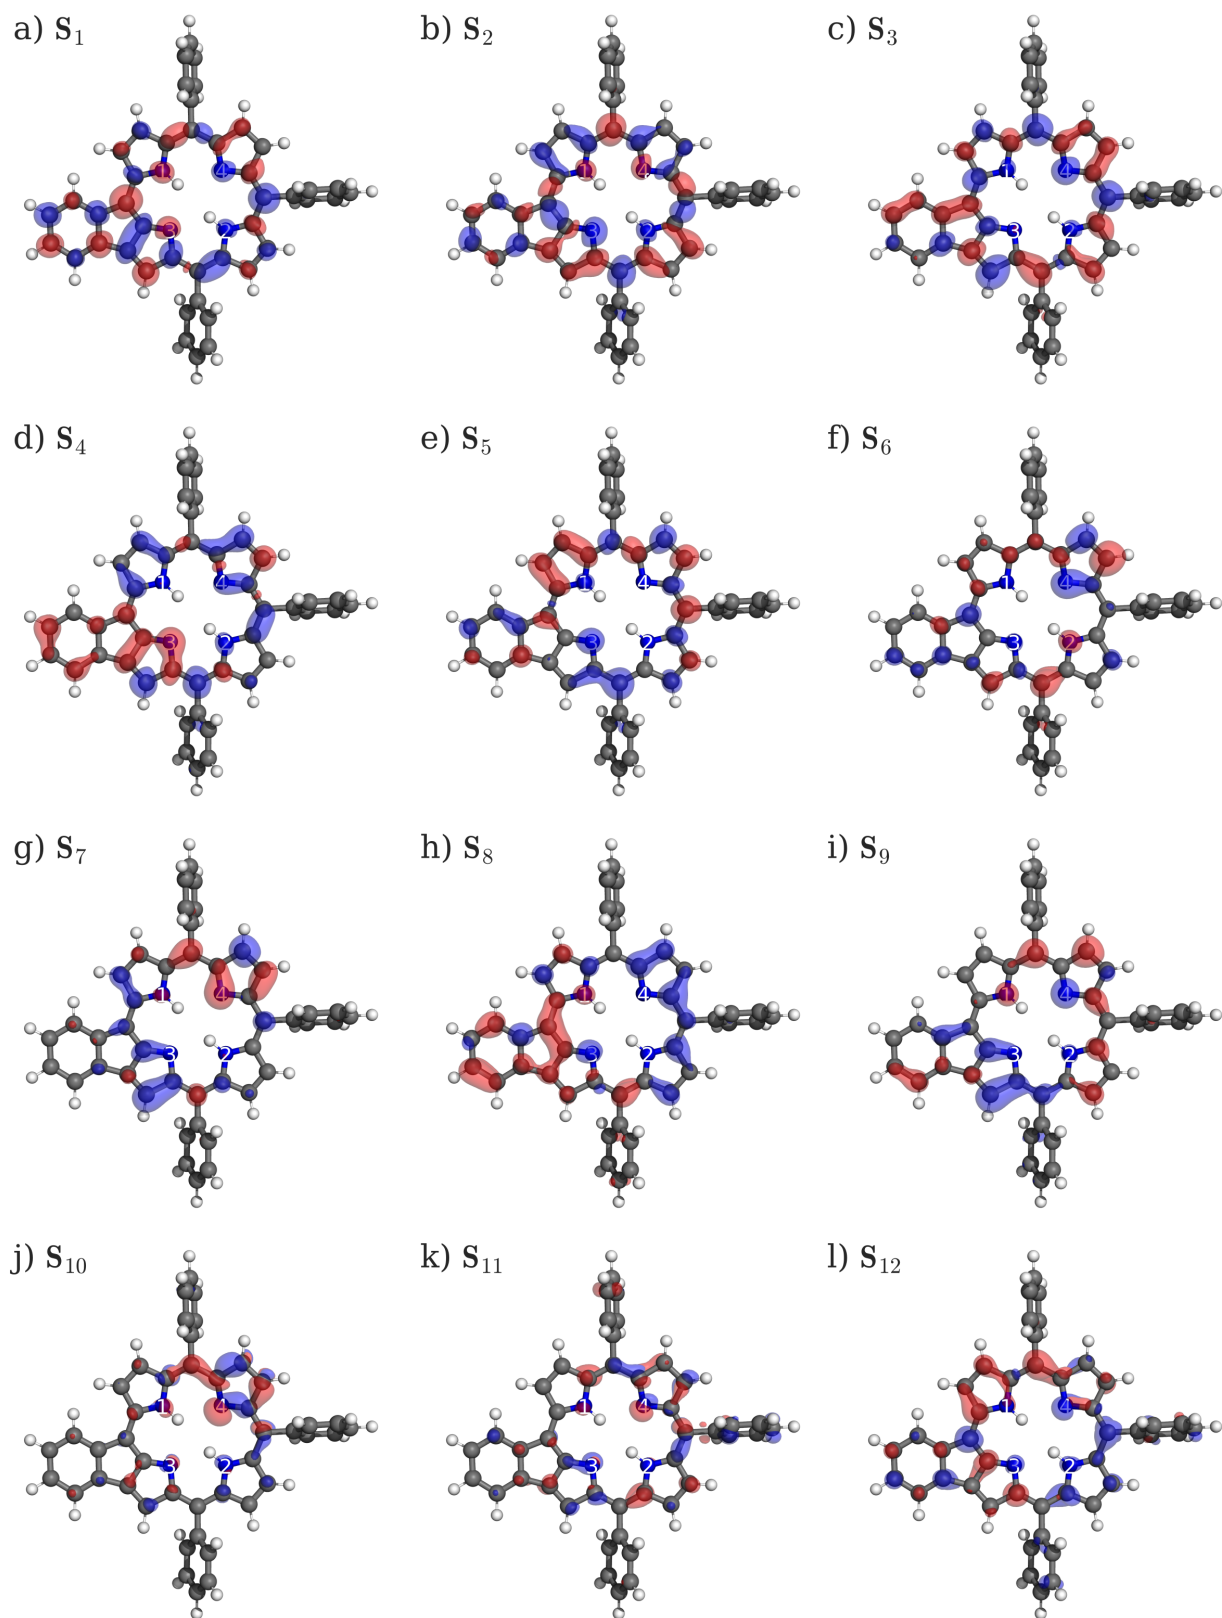

**Figure S2:** Transition densities of the 12 lowest RPA excitations in **5**.

**Table S2:** Dominant elements of the RPA eigenvectors vectors  $X_{ia}^\nu, Y_{ia}^\nu$  for the 12 lowest energy excitations in **5**. Listed are all elements which satisfy  $(X_{ia}^\nu + Y_{ia}^\nu)^2 > 0.01$ .

| $\nu$ | $i$ | $a$ | $X_{ia}^\nu + Y_{ia}^\nu$ | $\nu$ | $i$ | $a$ | $X_{ia}^\nu + Y_{ia}^\nu$ |
|-------|-----|-----|---------------------------|-------|-----|-----|---------------------------|
| 1     | 158 | 161 | 0.1072                    | 7     | 159 | 163 | -0.1281                   |
| 1     | 159 | 162 | 0.1707                    | 7     | 160 | 162 | -0.1116                   |
| 1     | 160 | 161 | 0.5939                    | 7     | 160 | 163 | -0.1909                   |
| 1     | 160 | 162 | -0.1933                   | 8     | 156 | 161 | 0.4566                    |
| 2     | 159 | 161 | 0.4377                    | 8     | 157 | 161 | 0.1120                    |
| 2     | 160 | 161 | -0.1241                   | 8     | 158 | 162 | -0.2411                   |
| 2     | 160 | 162 | -0.4929                   | 8     | 158 | 163 | 0.1026                    |
| 3     | 158 | 161 | -0.4744                   | 8     | 159 | 161 | 0.1602                    |
| 3     | 159 | 161 | 0.1826                    | 8     | 159 | 162 | -0.1810                   |
| 3     | 159 | 162 | 0.3870                    | 8     | 160 | 162 | 0.1140                    |
| 3     | 160 | 162 | 0.1627                    | 9     | 156 | 161 | 0.3066                    |
| 4     | 157 | 161 | -0.2314                   | 9     | 157 | 162 | -0.4754                   |
| 4     | 158 | 162 | 0.4658                    | 9     | 158 | 161 | -0.1287                   |
| 4     | 159 | 161 | 0.2828                    | 9     | 158 | 162 | 0.1837                    |
| 4     | 159 | 162 | -0.2119                   | 9     | 159 | 161 | -0.1117                   |
| 4     | 160 | 162 | 0.1642                    | 9     | 159 | 163 | -0.1220                   |
| 5     | 157 | 161 | -0.1880                   | 10    | 155 | 161 | 0.6687                    |
| 5     | 158 | 161 | -0.3002                   | 11    | 154 | 161 | -0.6768                   |
| 5     | 159 | 161 | -0.1325                   | 11    | 155 | 161 | 0.1052                    |
| 5     | 159 | 162 | -0.2204                   | 12    | 149 | 161 | 0.2088                    |
| 5     | 160 | 163 | 0.4848                    | 12    | 150 | 161 | -0.1740                   |
| 6     | 156 | 161 | 0.1101                    | 12    | 151 | 161 | 0.3371                    |
| 6     | 157 | 161 | -0.5885                   | 12    | 152 | 161 | 0.1609                    |
| 6     | 158 | 162 | -0.1561                   | 12    | 155 | 161 | -0.1426                   |
| 6     | 160 | 163 | -0.2459                   | 12    | 156 | 161 | -0.2401                   |
| 7     | 156 | 161 | 0.1749                    | 12    | 158 | 161 | -0.1398                   |
| 7     | 157 | 162 | 0.4547                    | 12    | 159 | 162 | -0.1583                   |
| 7     | 158 | 161 | -0.1267                   | 12    | 159 | 163 | -0.1674                   |
| 7     | 158 | 162 | 0.2674                    | 12    | 160 | 163 | -0.2307                   |
| 7     | 159 | 161 | -0.1424                   |       |     |     |                           |

### S3 Comparison to the satellite spectrum of the parent compounds

In Figure S3, we compare the first-order satellite spectra  $G_c^1(\omega)$  of the smaller molecules **1**, **5** and **6** with their parent compounds **2**, **3** and **4**. For the smaller molecules, we calculate the satellite spectrum using the fully analytical approach discussed in the main text

$$G_c^1(\omega) = \sum_v \frac{\gamma_c^v}{\omega - \epsilon_c^{\text{QP}} + \Omega^v + i\eta} \quad (\text{S1})$$

while in the numerical scheme, based on Eq. 13 of the main text, the first order satellite spectrum is approximated as

$$\text{Im}G_c^1(\omega + \epsilon_c^{\text{QP}}) \approx Z_c \frac{|\text{Im} \Sigma_c(\omega + \epsilon_c)|}{\pi \omega^2} \quad (\text{S2})$$

where  $\Sigma_c$  is the  $G_0W_0$  self-energy. All spectra are broadened using  $\eta = 0.1$  eV. The intensity of the most intense satellite is set to unity to facilitate comparison.

Now we discuss the differences in the satellite spectra introduced by using the simplified model systems **1**, **5** and **6** instead of the larger parent compounds **2**, **3** and **4**. Comparing **1** and **2**, we observe that the low-energy  $Q_{x/y}$  bands have the same intensity and position in both molecules. At higher energies, we see that for the N1/N2 the two peaks at 3.1 and 3.6 eV, which dominate the spectrum in **1**, split up in several peaks in compound **2**, although the overall intensity and the position of the maximum in the broadened spectrum is essentially the same. The spectra of the N3/N4 core-levels are very similar for both compounds.

For **3** and **5**, we find that the inclusion of the tert-butyl side-groups leads to an overall red-shift by roughly 0.1-0.2 eV. Furthermore, we observe that the relative peak ratio is altered, for example the  $S_1$  excitation in the N1 spectrum has a much lower intensity for **3** than in **5**, which is why it cannot be observed in Figure S1. Similar effects can be observed for **4** and **6**: Besides a general red-shift of 0.1-0.2 eV, we find that the spectrum of the parent compound exhibits a more complicated peak structure and in general different intensities than in the spectrum of the model compound **6**. For example, the intensity maximum in the N2 spectrum in **4** is dominated by several



transitions around 1.7-2.4 eV, while for **6** the same spectrum exhibits several additional peaks in the region between 2.5-2.9 eV.

Overall, we find that the spectra agree qualitatively well, which justifies the use of compounds **1**, **5** and **6** as model systems for their respective parent compounds. Still, quantitative predictions require the simulation of the full molecule.

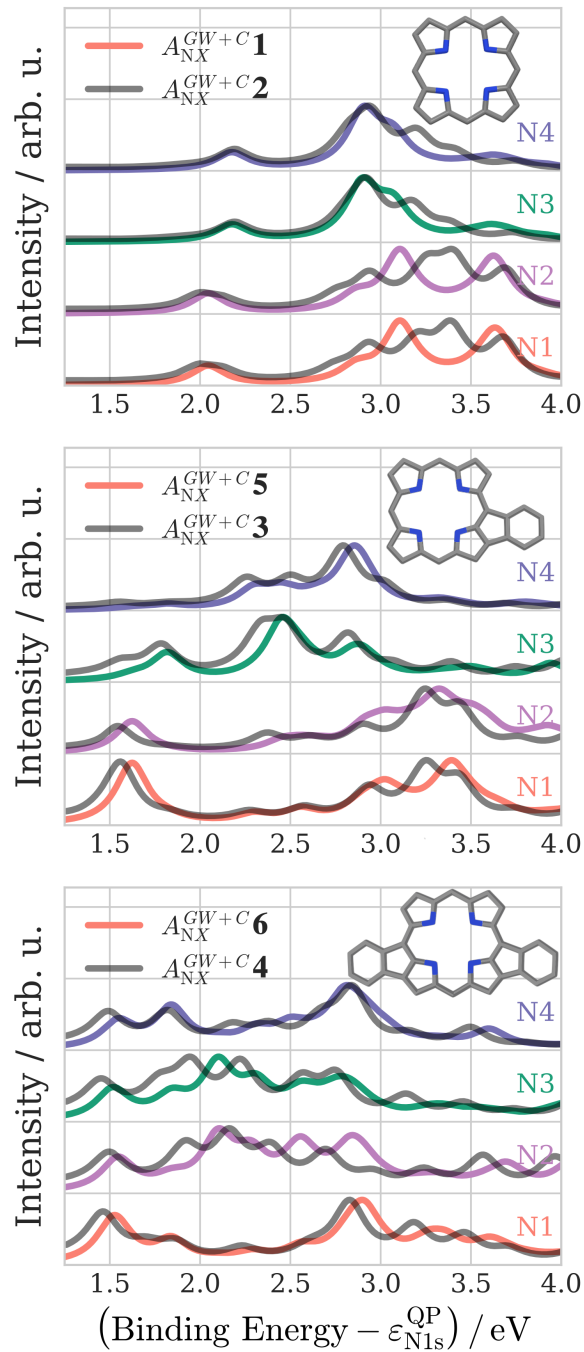

**Figure S3:** Comparison of the first order satellite spectrum  $G_{N1s}^1$  of the larger parent compounds **2**, **3** and **4** (black, computed based on Eq. 13 of the main text) to their smaller analogues **1**, **5** and **6** calculated using the fully analytical approach. The comparison is between the numerical satellite spectrum of the larger parent molecules and satellite spectrum of its smaller analogues, so between systems a) **1** and **2**, b) **3** and **5** and c) **4** and **6**. The defining macrocycle is sketched in the individual plots.

#### S4 UV-Vis spectrum of 1

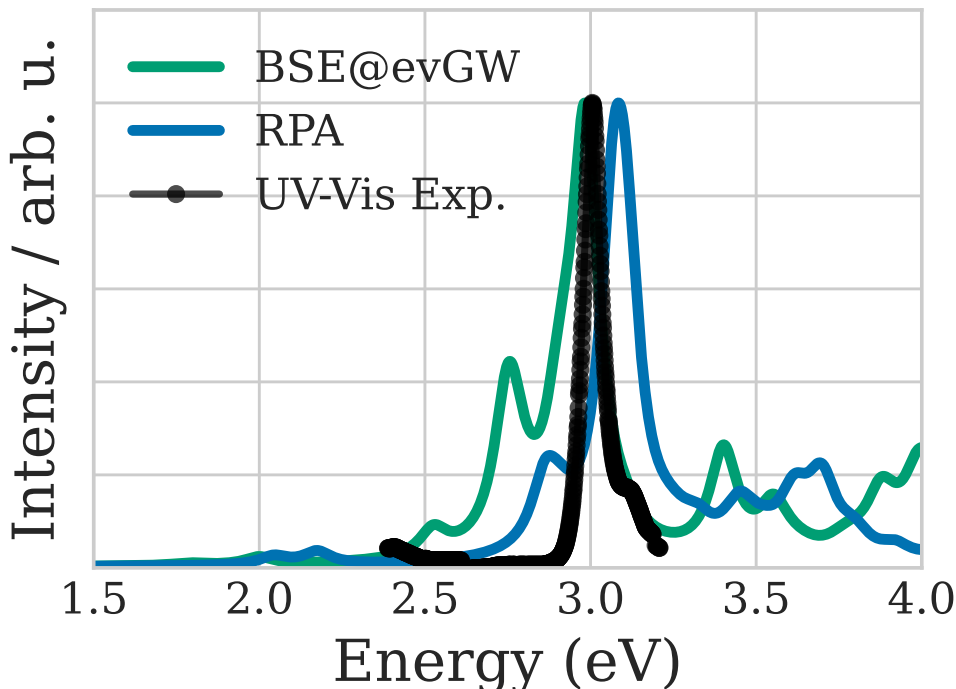

**Figure S4:** Comparison of the experimental UV-Vis spectrum of compound **2** (black, taken from Ref. S16) to the theoretical optical spectrum of molecule **1** in the RPA approximation (blue) and the more accurate BSE@evGW method (green).

In Figure S4, we compare the theoretical optical RPA spectrum of compound **1** to the higher level BSE@evGW and the experimental spectrum of **2** to assess the quality of the RPA approximation for the bound excitations in Porphyrins. We find that both calculations agree well with the experimental data and with each other. While the BSE@evGW spectrum is within 0.05 eV the experimental Soret band at 3.0 eV, the RPA approximation slightly overshoots by 0.2 eV. Comparing the RPA spectrum to the BSE@evGW data, we find the agreement very satisfying both in position and intensity of the bands. Both spectra exhibit a shoulder at the lower energy site, which is not present in the experimental data. Since the observed differences of ca.0.2 eV are below the experimental resolution for the shake-up satellites, we find that the use of RPA excitations is well justified for such systems.

## S5 RPA Excitations of 1

**Table S3:** RPA excitation energies  $\Omega^\nu$ , oscillator strengths  $f^\nu$  and  $GW + C$  satellite intensities  $\gamma_{N\chi}^\nu$  of the 30 lowest energy singlet excitations in **1**.

| $\nu$ | $\Omega^\nu / \text{eV}$ | $f^\nu$ | $\gamma_{N1}^\nu$ | $\gamma_{N2}^\nu$ | $\gamma_{N3}^\nu$ | $\gamma_{N4}^\nu$ |
|-------|--------------------------|---------|-------------------|-------------------|-------------------|-------------------|
| 1     | 2.0439                   | 0.0281  | 0.0195            | 0.0207            | 0.0000            | 0.0000            |
| 2     | 2.1745                   | 0.0425  | 0.0000            | 0.0000            | 0.0262            | 0.0287            |
| 3     | 2.8356                   | 0.0000  | 0.0000            | 0.0000            | 0.0000            | 0.0000            |
| 4     | 2.8632                   | 0.2121  | 0.0151            | 0.0158            | 0.0000            | 0.0000            |
| 5     | 2.8886                   | 0.0026  | 0.0000            | 0.0000            | 0.0493            | 0.0151            |
| 6     | 2.9070                   | 0.0857  | 0.0000            | 0.0000            | 0.0391            | 0.0788            |
| 7     | 3.0694                   | 0.9074  | 0.0001            | 0.0000            | 0.0515            | 0.0482            |
| 8     | 3.1055                   | 0.7342  | 0.0593            | 0.0610            | 0.0000            | 0.0000            |
| 9     | 3.1337                   | 0.0195  | 0.0006            | 0.0007            | 0.0008            | 0.0009            |
| 10    | 3.2155                   | 0.0186  | 0.0017            | 0.0005            | 0.0010            | 0.0000            |
| 11    | 3.2265                   | 0.0057  | 0.0010            | 0.0000            | 0.0001            | 0.0003            |
| 12    | 3.2420                   | 0.0153  | 0.0005            | 0.0009            | 0.0002            | 0.0001            |
| 13    | 3.2560                   | 0.0189  | 0.0001            | 0.0014            | 0.0001            | 0.0004            |
| 14    | 3.2713                   | 0.0086  | 0.0006            | 0.0002            | 0.0000            | 0.0009            |
| 15    | 3.2895                   | 0.0014  | 0.0000            | 0.0000            | 0.0002            | 0.0000            |
| 16    | 3.3028                   | 0.0163  | 0.0001            | 0.0012            | 0.0001            | 0.0017            |
| 17    | 3.3243                   | 0.0258  | 0.0000            | 0.0000            | 0.0002            | 0.0000            |
| 18    | 3.3262                   | 0.0325  | 0.0004            | 0.0001            | 0.0001            | 0.0000            |
| 19    | 3.3540                   | 0.0005  | 0.0005            | 0.0002            | 0.0000            | 0.0000            |
| 20    | 3.3874                   | 0.0005  | 0.0016            | 0.0003            | 0.0000            | 0.0001            |
| 21    | 3.3977                   | 0.0021  | 0.0006            | 0.0014            | 0.0000            | 0.0000            |
| 22    | 3.4043                   | 0.0003  | 0.0001            | 0.0000            | 0.0000            | 0.0001            |
| 23    | 3.4080                   | 0.0032  | 0.0000            | 0.0000            | 0.0001            | 0.0009            |
| 24    | 3.4165                   | 0.0051  | 0.0000            | 0.0001            | 0.0000            | 0.0002            |
| 25    | 3.4217                   | 0.0021  | 0.0000            | 0.0000            | 0.0001            | 0.0004            |
| 26    | 3.4340                   | 0.0229  | 0.0000            | 0.0003            | 0.0014            | 0.0000            |
| 27    | 3.4424                   | 0.0217  | 0.0001            | 0.0007            | 0.0000            | 0.0007            |
| 28    | 3.4446                   | 0.0138  | 0.0001            | 0.0001            | 0.0000            | 0.0006            |
| 29    | 3.4572                   | 0.0824  | 0.0002            | 0.0000            | 0.0001            | 0.0000            |
| 30    | 3.4865                   | 0.0017  | 0.0000            | 0.0009            | 0.0005            | 0.0002            |

**Table S4:** Dominant elements of the excitation vectors lowest ten excitations in **1**. Listed are all elements which satisfy  $(X_{ia}^\nu + Y_{ia}^\nu)^2 > 0.01$ .

| $\nu$ | $i$ | $a$ | $X_{ia}^\nu + Y_{ia}^\nu$ | $\nu$ | $i$ | $a$ | $X_{ia}^\nu + Y_{ia}^\nu$ |
|-------|-----|-----|---------------------------|-------|-----|-----|---------------------------|
| 1     | 160 | 163 | 0.5673                    | 8     | 157 | 162 | 0.1133                    |
| 1     | 161 | 162 | -0.7991                   | 8     | 158 | 162 | -0.5794                   |
| 2     | 160 | 162 | 0.5846                    | 8     | 159 | 164 | -0.1682                   |
| 2     | 161 | 163 | 0.7738                    | 8     | 160 | 163 | -0.4648                   |
| 3     | 158 | 164 | 0.1176                    | 8     | 161 | 162 | -0.2971                   |
| 3     | 159 | 162 | 0.9743                    | 8     | 161 | 171 | 0.1487                    |
| 4     | 158 | 162 | 0.7974                    | 9     | 154 | 162 | -0.1011                   |
| 4     | 160 | 163 | -0.4858                   | 9     | 156 | 163 | -0.1417                   |
| 4     | 161 | 162 | -0.2277                   | 9     | 157 | 163 | 0.5585                    |
| 5     | 158 | 163 | 0.1801                    | 9     | 161 | 164 | -0.7603                   |
| 5     | 159 | 163 | 0.9513                    | 10    | 154 | 163 | -0.1014                   |
| 6     | 158 | 163 | 0.8931                    | 10    | 155 | 162 | -0.1385                   |
| 6     | 159 | 163 | -0.1916                   | 10    | 156 | 162 | -0.5791                   |
| 6     | 160 | 162 | 0.2622                    | 10    | 156 | 163 | 0.1273                    |
| 6     | 161 | 163 | -0.1890                   | 10    | 157 | 162 | -0.6807                   |
| 7     | 148 | 163 | -0.2732                   | 10    | 157 | 163 | 0.3047                    |
| 7     | 149 | 162 | 0.2035                    | 10    | 160 | 164 | 0.1442                    |
| 7     | 150 | 163 | 0.1556                    | 11    | 154 | 162 | 0.2972                    |
| 7     | 156 | 162 | 0.1011                    | 11    | 154 | 163 | 0.1419                    |
| 7     | 158 | 163 | -0.4163                   | 11    | 156 | 162 | -0.6158                   |
| 7     | 160 | 162 | 0.6205                    | 11    | 156 | 163 | -0.1521                   |
| 7     | 161 | 163 | -0.3522                   | 11    | 157 | 162 | 0.5641                    |
| 7     | 161 | 172 | 0.1356                    | 11    | 157 | 163 | 0.2724                    |
| 8     | 148 | 162 | -0.2980                   | 11    | 160 | 164 | -0.1939                   |
| 8     | 149 | 163 | -0.1543                   | 11    | 161 | 164 | 0.1547                    |
| 8     | 150 | 162 | 0.1697                    | 12    | 155 | 162 | 0.9696                    |
| 8     | 154 | 162 | 0.1493                    | 12    | 156 | 163 | 0.1077                    |
| 8     | 155 | 162 | -0.1253                   |       |     |     |                           |

## S6 RPA Excitations of 6

**Table S5:** RPA excitation energies  $\Omega^\nu$ , oscillator strengths  $f^\nu$  and  $GW + C$  satellite intensities  $\gamma_{N\chi}^\nu$  of the 30 lowest energy singlet excitations in 6.

| $\nu$ | $\Omega^\nu / \text{eV}$ | $f^\nu$ | $\gamma_{N1}^\nu$ | $\gamma_{N2}^\nu$ | $\gamma_{N3}^\nu$ | $\gamma_{N4}^\nu$ |
|-------|--------------------------|---------|-------------------|-------------------|-------------------|-------------------|
| 1     | 1.5115                   | 0.0244  | 0.0224            | 0.0013            | 0.0240            | 0.0010            |
| 2     | 1.5463                   | 0.0280  | 0.0148            | 0.0186            | 0.0037            | 0.0278            |
| 3     | 1.8413                   | 0.0513  | 0.0168            | 0.0063            | 0.0185            | 0.0439            |
| 4     | 2.0986                   | 0.1230  | 0.0022            | 0.0312            | 0.0482            | 0.0052            |
| 5     | 2.2835                   | 0.0688  | 0.0058            | 0.0185            | 0.0003            | 0.0011            |
| 6     | 2.3102                   | 0.1035  | 0.0007            | 0.0003            | 0.0269            | 0.0154            |
| 7     | 2.4979                   | 0.0015  | 0.0000            | 0.0016            | 0.0004            | 0.0191            |
| 8     | 2.5558                   | 0.0536  | 0.0093            | 0.0236            | 0.0183            | 0.0010            |
| 9     | 2.6231                   | 0.0289  | 0.0006            | 0.0015            | 0.0048            | 0.0049            |
| 10    | 2.7371                   | 0.0386  | 0.0015            | 0.0008            | 0.0133            | 0.0069            |
| 11    | 2.7903                   | 0.0991  | 0.0001            | 0.0000            | 0.0058            | 0.0221            |
| 12    | 2.8146                   | 0.2628  | 0.0032            | 0.0039            | 0.0082            | 0.0221            |
| 13    | 2.8288                   | 0.2289  | 0.0108            | 0.0127            | 0.0032            | 0.0028            |
| 14    | 2.8520                   | 0.0285  | 0.0006            | 0.0055            | 0.0005            | 0.0008            |
| 15    | 2.8725                   | 0.2724  | 0.0006            | 0.0001            | 0.0057            | 0.0013            |
| 16    | 2.9109                   | 0.4151  | 0.0345            | 0.0100            | 0.0040            | 0.0206            |
| 17    | 2.9775                   | 0.0047  | 0.0000            | 0.0000            | 0.0002            | 0.0002            |
| 18    | 3.0145                   | 0.0144  | 0.0015            | 0.0001            | 0.0000            | 0.0056            |
| 19    | 3.0252                   | 0.0245  | 0.0014            | 0.0022            | 0.0017            | 0.0025            |
| 20    | 3.0420                   | 0.0957  | 0.0000            | 0.0002            | 0.0005            | 0.0046            |
| 21    | 3.1389                   | 0.0005  | 0.0000            | 0.0000            | 0.0001            | 0.0000            |
| 22    | 3.2004                   | 0.0866  | 0.0001            | 0.0019            | 0.0005            | 0.0009            |
| 23    | 3.2166                   | 0.0021  | 0.0014            | 0.0009            | 0.0012            | 0.0008            |
| 24    | 3.2357                   | 0.0087  | 0.0027            | 0.0002            | 0.0006            | 0.0003            |
| 25    | 3.2690                   | 0.0373  | 0.0091            | 0.0013            | 0.0038            | 0.0005            |
| 26    | 3.2894                   | 0.0003  | 0.0003            | 0.0001            | 0.0001            | 0.0002            |
| 27    | 3.3028                   | 0.0184  | 0.0001            | 0.0014            | 0.0003            | 0.0014            |
| 28    | 3.3212                   | 0.0172  | 0.0001            | 0.0005            | 0.0009            | 0.0001            |
| 29    | 3.3378                   | 0.0023  | 0.0002            | 0.0002            | 0.0000            | 0.0000            |
| 30    | 3.3485                   | 0.0330  | 0.0040            | 0.0023            | 0.0037            | 0.0024            |

**Table S6:** Dominant elements of the excitation vectors lowest ten excitations in **6**. Listed are all elements which satisfy  $(X_{ia}^\nu + Y_{ia}^\nu)^2 > 0.01$ .

| $\nu$ | $i$ | $a$ | $X_{ia}^\nu + Y_{ia}^\nu$ | $\nu$ | $i$ | $a$ | $X_{ia}^\nu + Y_{ia}^\nu$ |
|-------|-----|-----|---------------------------|-------|-----|-----|---------------------------|
| 1     | 157 | 160 | -0.1752                   | 8     | 157 | 160 | -0.3067                   |
| 1     | 158 | 160 | -0.7109                   | 8     | 157 | 161 | 0.1118                    |
| 1     | 158 | 161 | -0.2728                   | 8     | 159 | 162 | 0.3974                    |
| 1     | 159 | 160 | 0.5972                    | 9     | 151 | 160 | -0.1892                   |
| 2     | 158 | 160 | -0.6053                   | 9     | 155 | 160 | 0.2856                    |
| 2     | 158 | 161 | 0.3806                    | 9     | 156 | 160 | -0.1303                   |
| 2     | 159 | 160 | -0.5557                   | 9     | 157 | 161 | 0.4805                    |
| 2     | 159 | 161 | -0.3877                   | 9     | 158 | 162 | 0.7350                    |
| 3     | 156 | 160 | 0.1577                    | 10    | 152 | 160 | -0.2320                   |
| 3     | 157 | 160 | 0.3637                    | 10    | 153 | 160 | -0.3129                   |
| 3     | 158 | 160 | 0.2093                    | 10    | 154 | 160 | -0.5706                   |
| 3     | 158 | 161 | -0.2603                   | 10    | 155 | 161 | -0.2691                   |
| 3     | 159 | 161 | -0.8076                   | 10    | 156 | 161 | -0.5204                   |
| 3     | 159 | 162 | -0.1545                   | 10    | 156 | 162 | 0.1817                    |
| 4     | 155 | 160 | -0.1313                   | 10    | 157 | 161 | 0.1627                    |
| 4     | 156 | 160 | 0.6390                    | 10    | 157 | 162 | -0.1346                   |
| 4     | 157 | 160 | -0.2147                   | 10    | 158 | 162 | -0.1003                   |
| 4     | 157 | 161 | 0.2921                    | 10    | 158 | 167 | 0.1012                    |
| 4     | 158 | 161 | 0.5872                    | 11    | 151 | 160 | 0.1363                    |
| 4     | 158 | 162 | -0.1169                   | 11    | 152 | 160 | -0.2919                   |
| 4     | 159 | 160 | 0.1971                    | 11    | 153 | 160 | 0.7652                    |
| 4     | 159 | 161 | -0.1023                   | 11    | 155 | 161 | -0.3046                   |
| 5     | 156 | 160 | 0.1774                    | 11    | 156 | 160 | 0.1021                    |
| 5     | 156 | 161 | -0.1439                   | 11    | 157 | 160 | 0.1105                    |
| 5     | 157 | 160 | -0.5849                   | 11    | 157 | 161 | 0.2628                    |
| 5     | 157 | 161 | -0.1616                   | 11    | 157 | 162 | 0.1406                    |
| 5     | 158 | 161 | -0.1903                   | 11    | 159 | 162 | -0.1300                   |
| 5     | 158 | 162 | 0.1921                    | 12    | 146 | 160 | 0.1084                    |
| 5     | 159 | 160 | -0.1160                   | 12    | 147 | 160 | -0.1348                   |
| 5     | 159 | 162 | -0.6657                   | 12    | 151 | 160 | 0.3401                    |
| 6     | 155 | 160 | -0.1156                   | 12    | 152 | 160 | 0.1731                    |
| 6     | 156 | 160 | -0.6654                   | 12    | 153 | 160 | -0.4900                   |
| 6     | 157 | 160 | -0.1599                   | 12    | 154 | 160 | 0.2400                    |
| 6     | 157 | 161 | 0.3681                    | 12    | 154 | 161 | 0.2369                    |
| 6     | 158 | 161 | 0.2352                    | 12    | 155 | 160 | -0.1150                   |
| 6     | 158 | 162 | -0.3675                   | 12    | 155 | 161 | -0.2465                   |
| 6     | 159 | 160 | 0.1204                    | 12    | 156 | 160 | 0.1353                    |
| 6     | 159 | 161 | -0.1137                   | 12    | 156 | 161 | 0.2003                    |
| 6     | 159 | 162 | -0.3320                   | 12    | 157 | 161 | 0.3647                    |
| 7     | 155 | 160 | 0.8894                    | 12    | 157 | 162 | 0.2434                    |
| 7     | 157 | 160 | -0.1015                   | 12    | 158 | 161 | -0.1810                   |
| 7     | 158 | 162 | -0.3871                   | 12    | 158 | 162 | -0.1546                   |
| 8     | 154 | 160 | 0.5369                    | 12    | 159 | 160 | -0.1033                   |
| 8     | 155 | 160 | -0.1206                   | 12    | 159 | 162 | -0.1200                   |
| 8     | 156 | 161 | -0.6022                   |       |     |     |                           |

## S7 Experimental fit parameters

### S7.1 XP spectrum of H2-TPP (1)

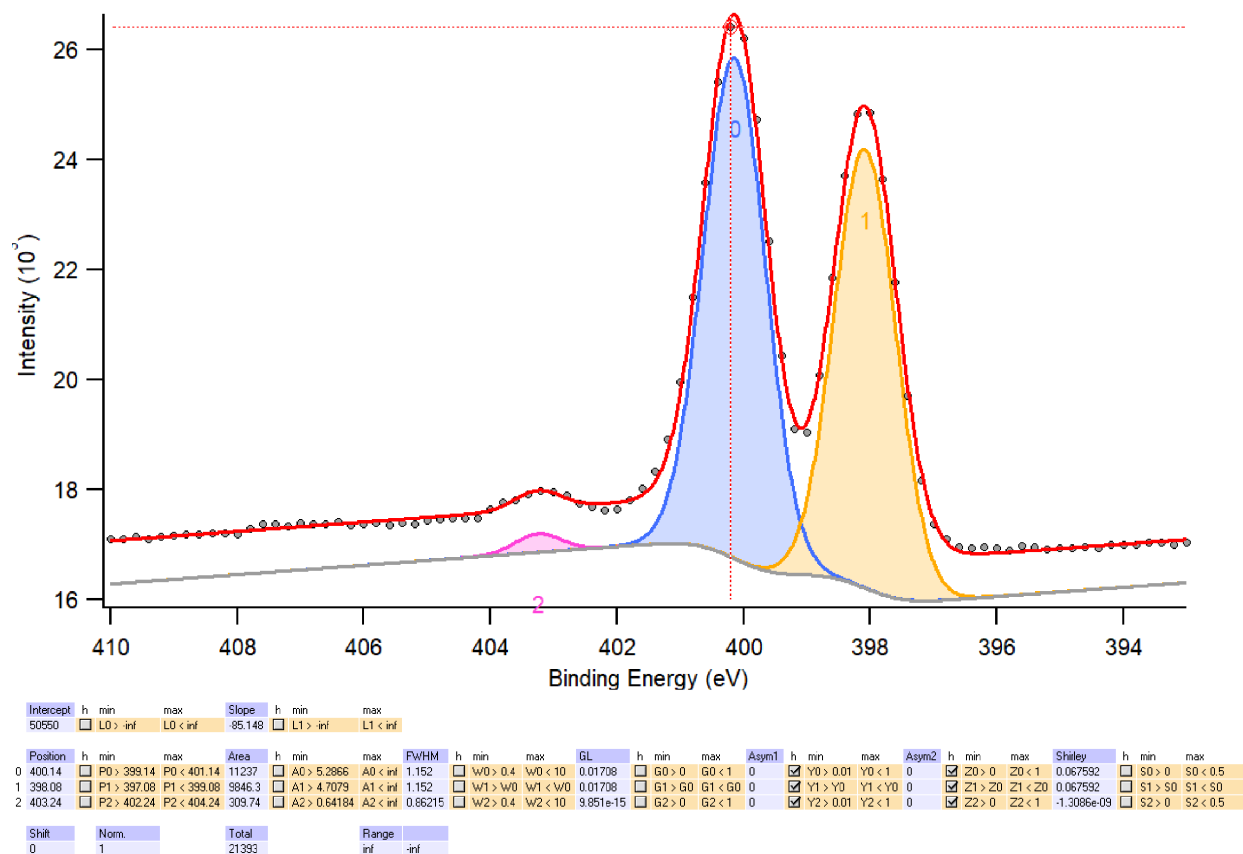

Figure S5: Experimental XPS fit data of compound 1.



## S7.2 XP spectrum of 2

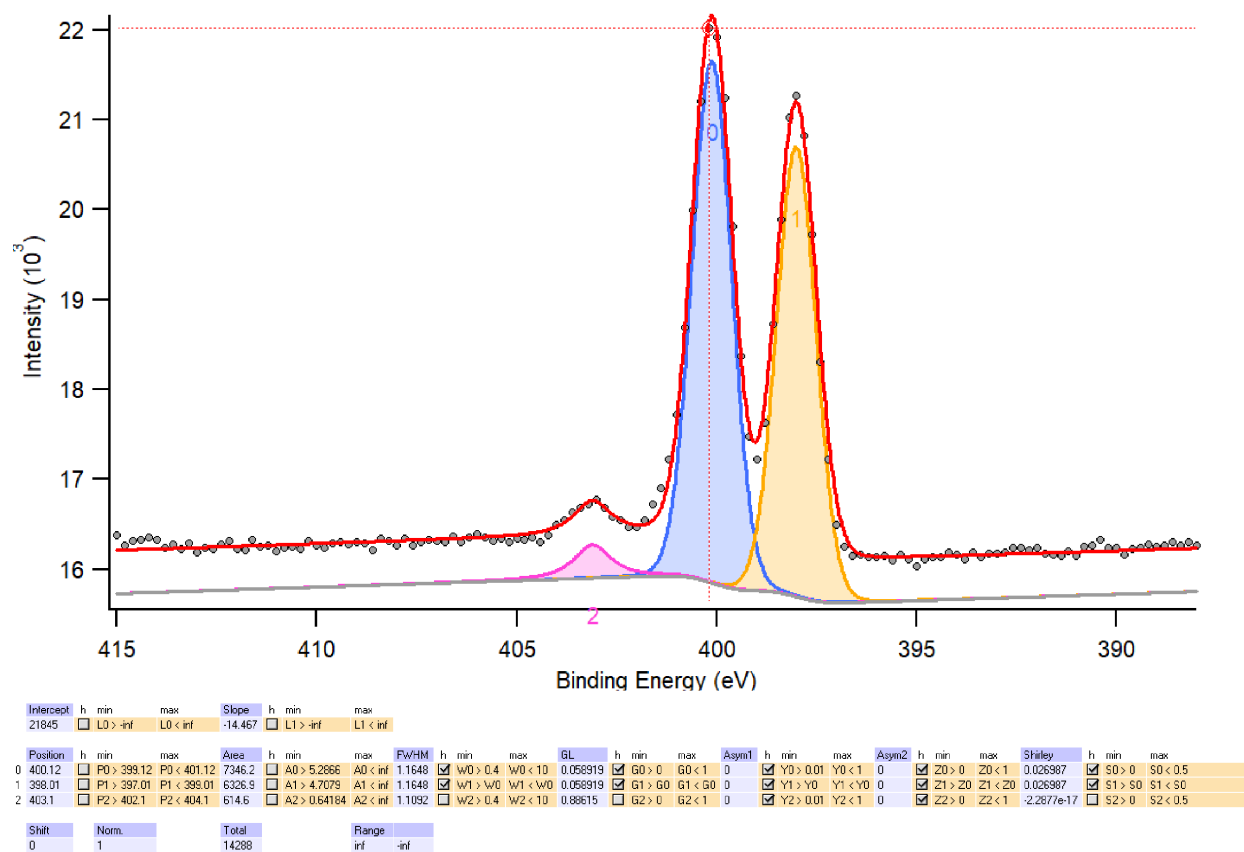

Figure S6: Experimental XPS fit data of compound 2.

### S7.3 XP spectrum of 3

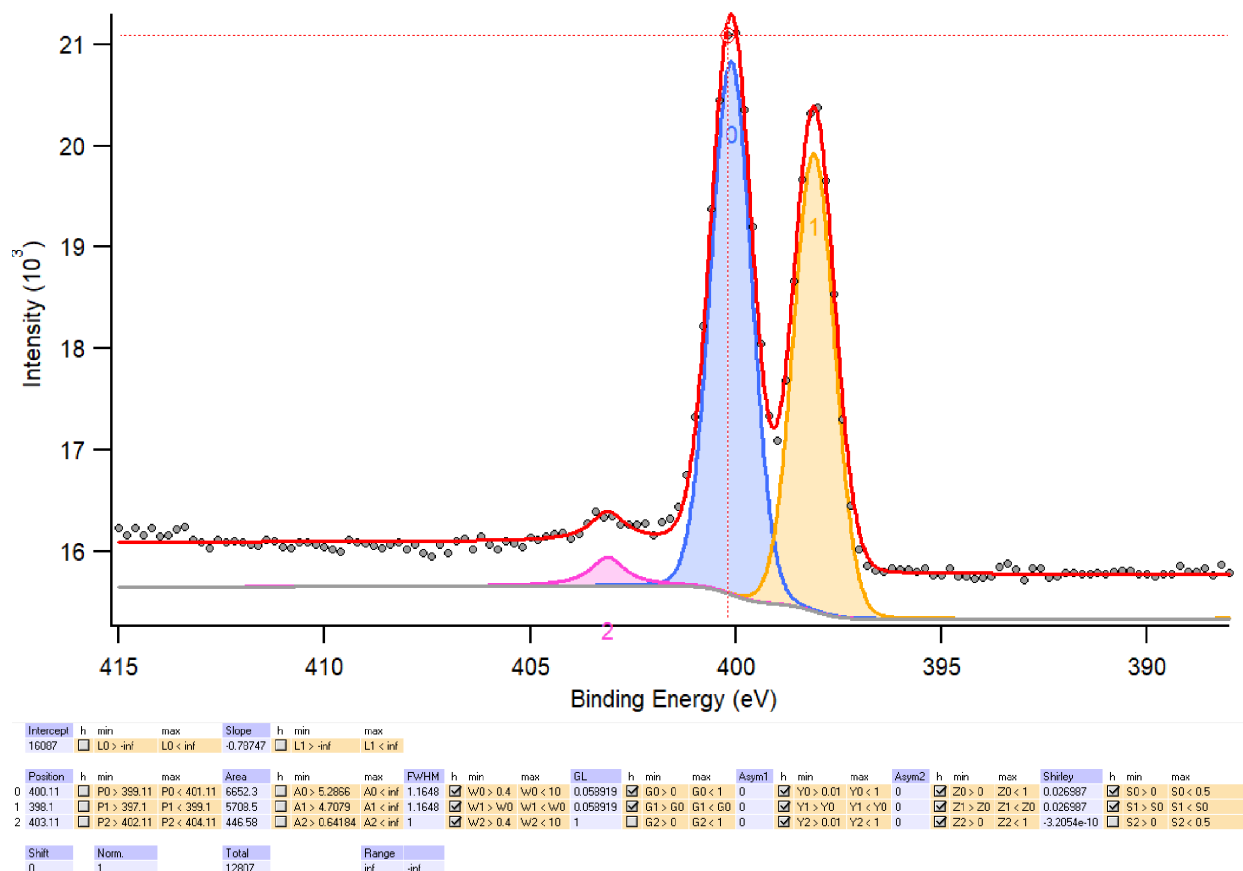

Figure S7: Experimental XPS fit data of compound 3.

## References

- [S1] Blum, V.; Gehrke, R.; Hanke, F.; Havu, P.; Havu, V.; Ren, X.; Reuter, K.; Scheffler, M. Ab initio molecular simulations with numeric atom-centered orbitals. *Comput. Phys. Commun.* **2009**, *180*, 2175–2196.
- [S2] Ren, X.; Rinke, P.; Blum, V.; Wieferink, J.; Tkatchenko, A.; Sanfilippo, A.; Reuter, K.; Scheffler, M. Resolution-of-identity approach to Hartree–Fock, hybrid density functionals, RPA, MP2 and GW with numeric atom-centered orbital basis functions. *New J. Phys.* **2012**, *14*, 053020.

- [S3] Abbott, J. W.; Acosta, C. M.; Akkoush, A.; Ambrosetti, A.; Atalla, V.; Bagrets, A.; Behler, J.; Berger, D.; Bieniek, B.; Björk, J.; others Roadmap on advancements of the FHI-aims software package. *arXiv preprint arXiv:2505.00125* **2025**,
- [S4] Kockläuner, J.; Golze, D. *GW* plus cumulant approach for predicting core-level shakeup satellites in large molecules. *J. Chem. Theory Comput.* **2025**, *21*, 3101–3119.
- [S5] Li, J.; Jin, Y.; Rinke, P.; Yang, W.; Golze, D. Benchmark of *GW* methods for core-level binding energies. *J. Chem. Theory Comput.* **2022**, *18*, 7570–7585.
- [S6] Perdew, J. P.; Burke, K.; Ernzerhof, M. Generalized gradient approximation made simple. *Phys. Rev. Lett.* **1996**, *77*, 3865.
- [S7] Tkatchenko, A.; Scheffler, M. Accurate Molecular Van Der Waals Interactions from Ground-State Electron Density and Free-Atom Reference Data. *Phys. Rev. Lett.* **2009**, *102*, 073005.
- [S8] Golze, D.; Wilhelm, J.; Van Setten, M. J.; Rinke, P. Core-level binding energies from *GW*: An efficient full-frequency approach within a localized basis. *J. Chem. Theory Comput.* **2018**, *14*, 4856–4869.
- [S9] Panadés-Barrueta, R. L.; Golze, D. Accelerating core-level *GW* calculations by combining the contour deformation approach with the analytic continuation of *W*. *J. Chem. Theory Comput.* **2023**, *19*, 5450–5464.
- [S10] Liu, C.; Kloppenburg, J.; Yao, Y.; Ren, X.; Appel, H.; Kanai, Y.; Blum, V. All-electron *ab initio* Bethe-Salpeter equation approach to neutral excitations in molecules with numeric atom-centered orbitals. *J. Chem. Phys.* **2020**, *152*.
- [S11] Yao, Y.; Golze, D.; Rinke, P.; Blum, V.; Kanai, Y. All-electron BSE@ *GW* method for K-edge core electron excitation energies. *J. Chem. Theory Comput.* **2022**, *18*, 1569–1583.

- [S12] Krause, K.; Klopper, W. Implementation of the Bethe- Salpeter equation in the TURBO- MOLE program. 2017.
- [S13] van Setten, M. J.; Weigend, F.; Evers, F. The GW-method for quantum chemistry applica- tions: Theory and implementation. *J. Chem. Theory Comput.* **2013**, *9*, 232–246.
- [S14] Kaplan, F.; Harding, M. E.; Seiler, C.; Weigend, F.; Evers, F.; van Setten, M. J. Quasi- particle self-consistent GW for molecules. *J. Chem. Theory Comput.* **2016**, *12*, 2528–2541.
- [S15] Franzke, Y. J.; Holzer, C.; Andersen, J. H.; Begusic, T.; Bruder, F.; Coriani, S.; Della Sala, F.; Fabiano, E.; Fedotov, D. A.; Fuürst, S.; others TURBOMOLE: Today and tomorrow. *J. Chem. Theory Comput.* **2023**, *19*, 6859–6890.
- [S16] Oleszak, C.; Schol, P. R.; Ritterhoff, C. L.; Krug, M.; Martin, M. M.; Bo, Y.; Meyer, B.; Clark, T.; Guldi, D. M.; Jux, N. Fused Hexabenzocoronene-Porphyrin Conjugates with Tai- lorable Excited-State Lifetimes. *Angew. Chem.* **2024**, *136*, e202409363.
